# Supplementary material for: Semantic Palette: Guiding Scene Generation with Class Proportions
Source: arXiv:2106.01629 source file (2021-06-03)
Supplement: Supplementary file 1 [file transport.pdf]

**Semantic Palette**

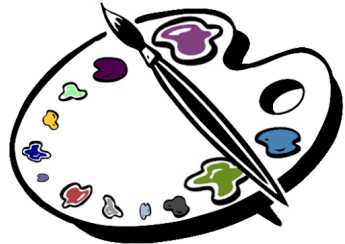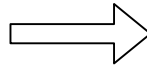

**Well-proportioned spatially-uniform semantic map**

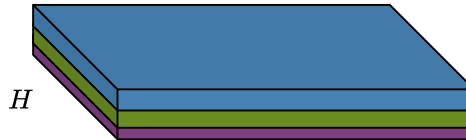

$$\frac{1}{HW}$$

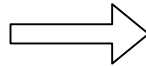

**Generated semantic map**

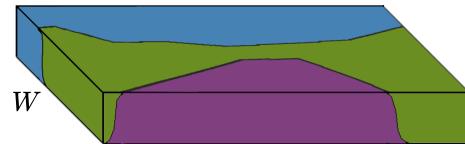

$$\frac{1}{HW}$$
